# Supplementary material for: Hyperfine-Structure-Induced Depolarization of Impulsively Aligned $\rm I_2$ Molecules
Source: arXiv:1804.04416 ancillary file (2018-04-12)
Supplement: Supplementary file 1 [file SM_HyperfineI2-hs.pdf]

# Supplemental Material

# Hyperfine-structure-induced depolarization of impulsively aligned $I_2$ molecules

Esben F. Thomas,[1] Anders A. Søndergaard,[2] Benjamin Shepperson,[2] Niels E. Henriksen,[1] and Henrik Stapelfeldt[2]

[1]*Department of Chemistry, Technical University of Denmark, Building 206, DK-2800 Kongens Lyngby, Denmark*

[2]*Department of Chemistry, Aarhus University, Langelandsgade 140, DK-8000 Aarhus C, Denmark*

(Dated: April 12, 2018)

**CONTENTS**

Are experimental factors influencing the observed alignment dynamics? 3

Simulation with centrifugal distortion 4

Simulation with fitted temperature 6

Analysis of the impact of the vibrational temperature 7

Simulation of high-$J$ wavepacket to 1 $\mu$s 10

References 12

## ARE EXPERIMENTAL FACTORS INFLUENCING THE OBSERVED ALIGNMENT DYNAMICS?

Firstly, the conditions of the molecular beam used were such that there was absolutely no collisions between the $I_2$ molecules and other molecules or atoms on the nanosecond observation time of the experiment [1].

Secondly, the maximum delay of the probe pulse with respect to the kick pulse was 3.2 ns (see Fig. 1 in the main text). With a speed of about 1700 m/s (determined by the helium carrier gas in the supersonic expansion) the $I_2$ molecules moved a maximum of 3.2 ns $\times$ 1700 m/s = 5.4 $\mu$m between the kick pulse and the probe pulse. The probe laser beam and the kick laser beam were spatially overlapped in the experiment and their Gaussian spotsizes were $\omega_0(\text{kick}) = 25$ $\mu$m and $\omega_0(\text{kick}) = 35$ $\mu$m. This ensured that the probe pulse actually probed molecules that had been aligned by the kick pulse. If the delay had been increased to e.g. 10 ns or more it would have been necessary to spatially offset the focus of the probe beam downstream of the molecular beam.

Thirdly, the extraction field in the VMI spectrometer is about 500 V/cm. Since $I_2$ is nonpolar there were no interaction with a possible dipole moment. In addition, the interaction between the extraction field and the polarizability of the molecules is negligible.

We conclude that none of the three experimental factors influence the observed alignment dynamics.

## SIMULATION WITH CENTRIFUGAL DISTORTION

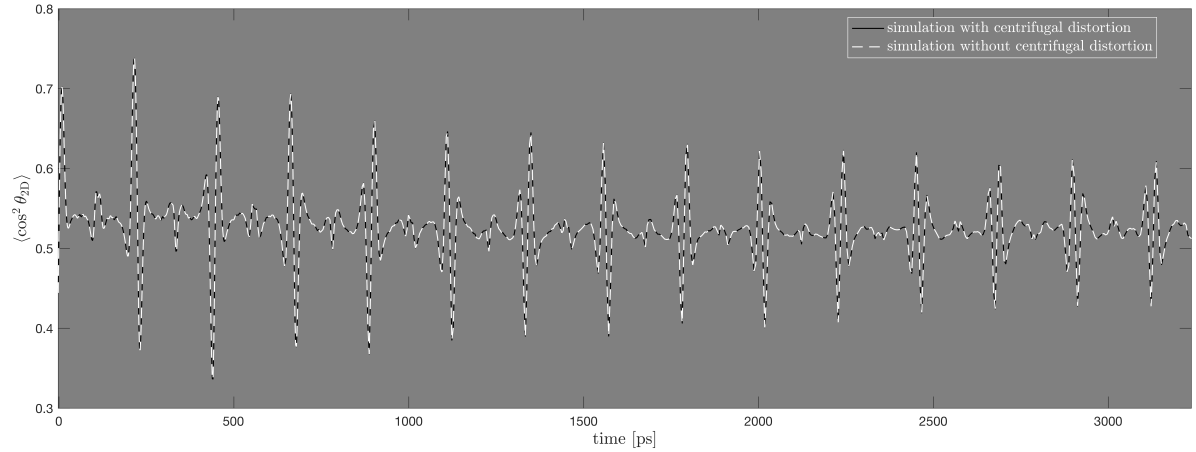


Figure 1. Overlaid simulated quadrupole coupled traces with (black solid line) and without (white dashed line) the effects of centrifugal distortion included. The background color has been darkened to enhance the contrast between the two traces since they are nearly identical.

Centrifugal distortion leads to a decrease in the energy spacing of the rotational energy levels as a function of $J$. It is one of the well-known ways that the behaviour of a real molecule will deviate from the rigid rotor approximation, and its effect on our quantum mechanical model is therefore worth investigating. The effects of centrifugal distortion can be included in our model by modifying the rotational energy as a function of $J$ in the following way:

$$E_J = B_0 J(J+1) - D_0 J^2 (J+1)^2, \tag{1}$$

where $B_0 = 1.11863$ GHz and $D_0 = 67.7531$ Hz are, respectively, the molecular rotational constant and centrifugal distortion constant of $I_2$ in the vibrational ground state [2]. A rough calculation shows that the size of the centrifugal correction term will be comparable to that of the $B_0$ constant when $J \approx 50$. In a sense this means that we should not expect centrifugal distortion to play a significant role when $J < 50$.

The average $J$ value in the rotational wave packets generated by our experimental pulse is about 5, so based on our rough analysis we are very far from the threshold where centrifugal distortion will play a role. Nevertheless, a simulation was performed where the centrifugal correction term was added to $\mathcal{H}_B$ in Eq. (2) of the main article text. The result of this

simulation is overlaid with the simulation performed without centrifugal distortion in Fig. 1, and as expected the two traces are almost completely identical. This underlines that the deviations from the rigid rotor model observed in the experimental trace are in no meaningful way associated with the effect of centrifugal distortion.

## SIMULATION WITH FITTED TEMPERATURE

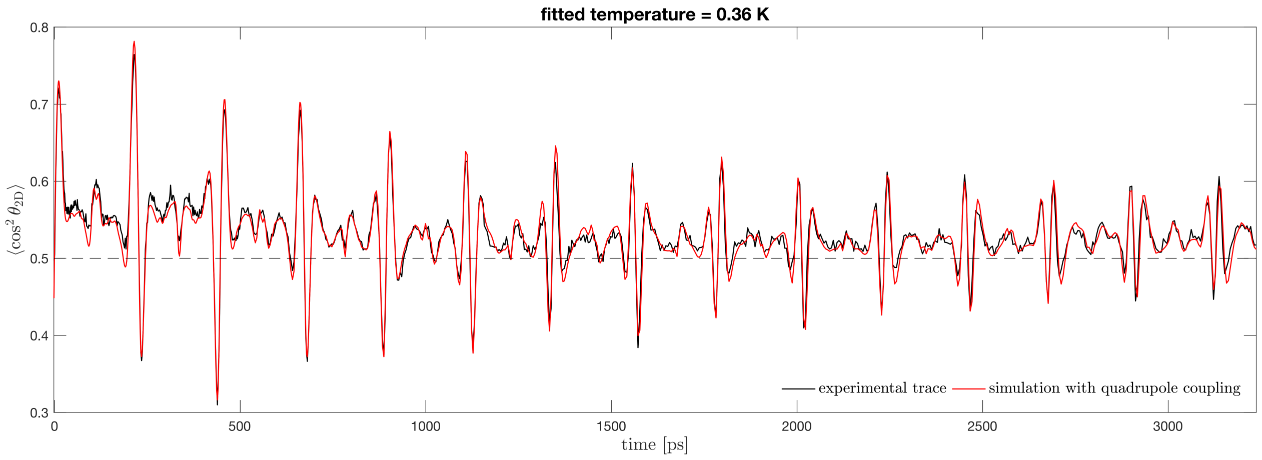


Figure 2. Experimental results (black) and the model calculations (red) calculated using a fitted initial rotational temperature of $T = 0.36$ K.

As stated in the main article text, fitting the simulated initial rotational temperature to minimize the RMSE will lead to a simulated trace that agrees better with the experimental data during the initial 600 ps. This result can be seen in Fig. 2, where the fitted temperature was found to be 0.36 K. Note that the agreement at times after 600 ps is roughly the same as in the 0.8 K case shown in Fig. 1 of the main article.

Generally, it was found that using simulated temperatures in the range of $\sim 0.3 - 1$ K would lead to good agreement between the theoretical and experimental traces at times after 600 ps. This gives credence to the conclusion that the observed deviations from the rigid rotor approximation are specifically due to quadrupole coupling, and not a result of parametric overfitting.

## ANALYSIS OF THE IMPACT OF THE VIBRATIONAL TEMPERATURE

The molecular beam in our experiments is created by expanding $\sim 1$ mbar iodine gas in 80 bar of He gas into vacuum through an Even Lavie valve. As mentioned in the main text this leads to a rotational temperature of about 1 K. Such low rotational temperatures have been reported for several other molecules [3, 4] and it has also been shown that the high pressure expansion leads to strong vibrational cooling [3]. As such we expected that most of the $I_2$ molecules reside in the vibrational ground state prior to the kick pulse. Nevertheless, since we do not have a precise estimate for the vibrational temperature in the experiment, in this section we investigate how molecules in the first excited vibrational state influence the alignment dynamics.

At temperatures from $0 - 300$ K, only the first two vibrational states, $\nu_0$ and $\nu_1$, have the potential to be significantly populated. $I_2$ in the $\nu_1$ vibrational state (hereby denoted $I_2^{\nu_1}$) has a rotational constant that is slightly smaller ($\sim 0.3\%$) than the rotational constant of $I_2$ in the vibrational ground state ($I_2^{\nu_0}$). This means that in general the alignment trace of $I_2^{\nu_1}$ will be slightly "stretched" compared to that of $I_2^{\nu_0}$. Therefore, an incoherent superposition of $I_2^{\nu_1}$ and $I_2^{\nu_0}$ traces will initially start to destructively (and later constructively) interfere over time as they move out of (and back into) phase with each other. Qualitatively, the initial destructive interference will manifest itself as an attenuation of the peak height in the $\langle \cos^2 \theta_{2D} \rangle_{coh}$ component of the alignment trace.

Effectively, the introduction of higher vibrational states will have some of the same qualitative effects on the alignment trace as that of the quadrupole coupling (decreasing the peak amplitude over time). The question that must be answered is therefore how much of the observed peak attenuation is due to quadrupole coupling, and how much is potentially due to $I_2$ molecules in higher vibrational states?

To this end, we performed simulations of the quadrupole and non-quadrupole coupled systems, where all parameters were the same except the rotational constant was modified to that of $I_2^{\nu_1}$ (the $eqQ$ quadrupole coupling constant for $I_2^{\nu_1}$ can safely be assumed to be identical to that of $I_2^{\nu_0}$ [5]). We then incoherently added the $I_2^{\nu_1}$ traces to the $I_2^{\nu_0}$ traces to reflect thermal vibrational distributions from $0 - 300$ K. Results for vibrational temperatures of 1, 100, 200 and 300 K are shown with and without quadrupole coupling and compared to the experimental results in Fig. 3 for trace structures appearing between 2600 and 3200 ps

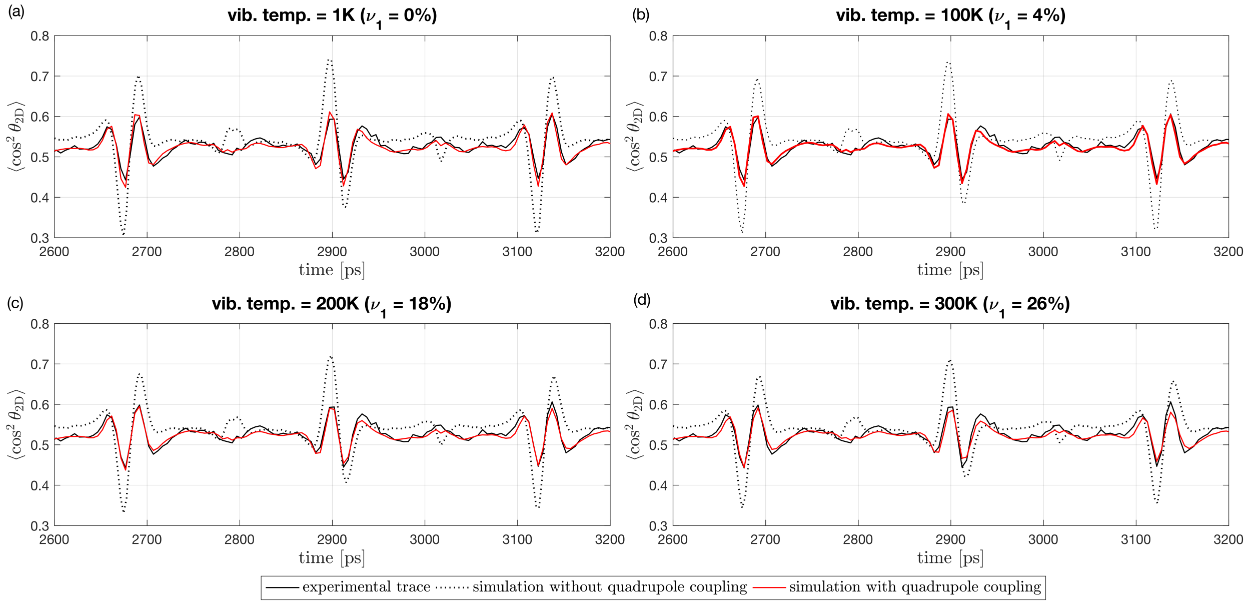


Figure 3. Close-up view of the $n = 6 - 7$ revival peaks appearing between 2600 and 3200 ps. calculated at various vibrational temperatures with (red line) and without (dotted line) quadrupole coupling, compared to the experimental trace (black line). In (a) we assume that the vibrational temperature is roughly the same as the rotational temperature, i.e. only the ground vibrational state $\nu_0$ is populated and the trace is identical to the one appearing in Fig. 1 of the main article. In (b), (c) and (d) we incoherently sum traces calculated for $I_2$ molecules in $\nu_0$ and $\nu_1$ vibrational states with proportions corresponding to Boltzmann distributions at 100, 200 and 300 K, respectively.

(we focus on this region of the trace because the attenuating effect of the higher vibrational states only becomes significant at longer time scales).

While close inspection of Fig. 3 indicates that vibrational temperatures from $100 - 300$ K will have a small impact on the peak amplitudes of both the quadrupole coupled and non-quadrupole coupled traces, it is clear that the quadrupole coupling plays the dominant role in modulating the overall amplitude and/or structure of the trace. In particular, the pronounced changes of the shape of the quarter revivals can only be accounted for by the quadrupole coupling.

It is also in principle possible that the kick pulse causes some excitation from the vibrational ground state to the first excited vibrational state through a stimulated Raman transition. In Ref. [6], the authors simulate hitting $Cl_2$ molecules in the vibrational ground state with transform limited pulses where the widths have been optimized to induce vibra-

tional transitions. Even though the simulated intensities are about $10\times$ higher than our experimental pulse, this only leads to a $\nu_1$ population of about 0.1%. The derivative of the polarizability function at the equilibrium bond distance (and therefore the Raman transition probability) of $I_2$ is similar to that of $Cl_2$ [7, 8], so the results from Ref. [6] strongly indicate that it is unlikely that any significant vibrational excitation is caused by our experimental pulse.

## SIMULATION OF HIGH-$J$ WAVEPACKET TO 1 $\mu$s

As stated in the main article text, it is already well understood from, e.g., the classical illustration in Ref. [9], that if $|J|$ is much larger than $|I|$ then the relative change in the projection $M_J$ along the $z$ axis as $\mathbf{I}$ and $\mathbf{J}$ precess around $\mathbf{F}$ will be insignificant, putting an absolute limit on how much depolarization will occur in $\langle\cos^2\theta_{2\mathrm{D}}\rangle_{\mathrm{perm}}$. As we uncover in our analysis, this is not the case for $\langle\cos^2\theta_{2\mathrm{D}}\rangle_{\mathrm{coh}}$, where it is posited that peak structures will eventually decay to the same "background" level regardless of the magnitude of the $J$ values present in the rotational wave packet (although the size of the $J$'s is associated with how long the decay takes).

In the main text we test this claim by creating wave packets with larger $J$, by increasing the simulated pulse intensity. In this supporting section, we go further by upping the intensity to 10 TW/cm$^2$, over 9 times the experimental value, creating a rotational wave packet with an average $J$ value of 39, almost 8 times larger than the biggest $I$ value (5) present in the system.

The decay of the peak structures in $\langle\cos^2\theta_{2\mathrm{D}}\rangle_{\mathrm{coh}}$ will happen very slowly in this case, so it is computationally unfeasible to simulate the entire alignment trace until the peaks disappear. Fortunately, the properties of our simulation allow us to jump forward to any time interval without having to calculate the preceding dynamics. Fig. 4 shows the simulated alignment trace in 500 ps segments beginning at 0, 200, 500, and 1000 ns. It can be clearly seen that the revival peak structures are almost completely gone by 1000 ns, whereas the change in the permanent (average) alignment from the initial level is very small.

This result further serves to underline one of the aforementioned main qualitative differences between how the quadrupole coupling affects the $\langle\cos^2\theta_{2\mathrm{D}}\rangle_{\mathrm{coh}}$ and $\langle\cos^2\theta_{2\mathrm{D}}\rangle_{\mathrm{perm}}$ components of the alignment trace for rotational wave packets in the high $J$ limit; the effect on $\langle\cos^2\theta_{2\mathrm{D}}\rangle_{\mathrm{perm}}$ becomes negligible whereas the effect on $\langle\cos^2\theta_{2\mathrm{D}}\rangle_{\mathrm{coh}}$ always eventually becomes significant (as a side note, it is clear the time scales where this happens can potentially become so long that they are not feasible to measure in a given experimental setup).

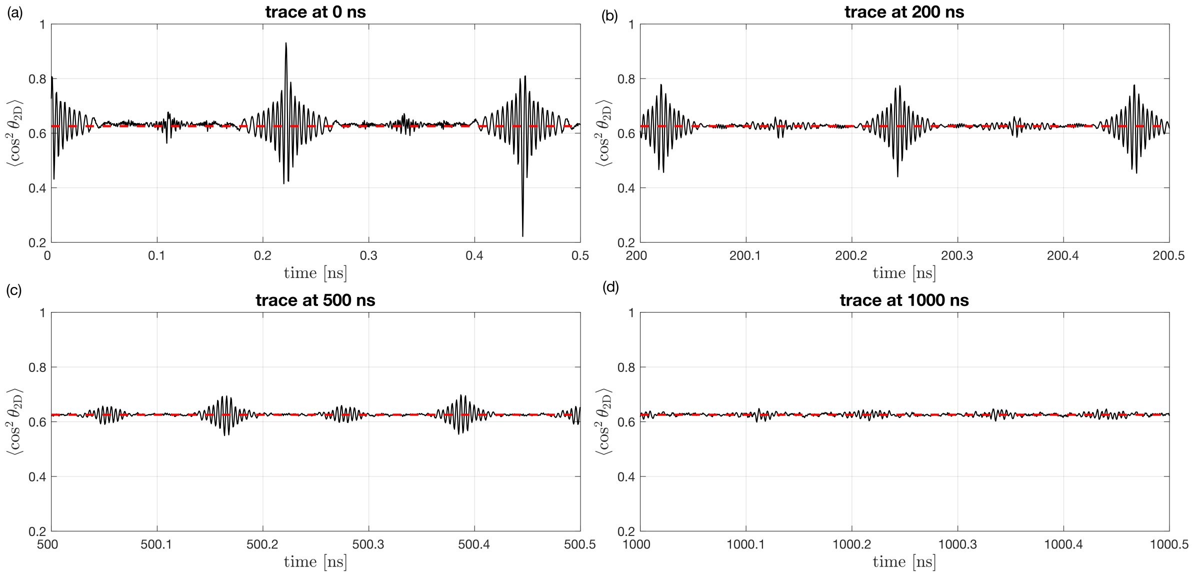


Figure 4. Quadrupole-coupled alignment trace simulated in 500 ps intervals starting at 0, 200, 500, and 1000 ns, using an alignment pulse intensity of 10 $TW/cm^2$. A pulse of this intensity yields a system of rotational wave packets where the average $J$ value is 39, significantly larger than the $I$ values present in the system. The horizontal red dashed lines are set to the mean of the trace values calculated at 500 and 1000 ns, and are meant to serve as visual aids to illustrate how little the average level of alignment deviates from its initial value over time. Note that because of the large $J$ states present here, we have included centrifugal distortion in our simulation.

[1] D. M. Lubman, C. T. Rettner, and R. N. Zare. How isolated are molecules in a molecular beam? *J. Phys. Chem.*, 86:1129, 1982.

[2] P.J. Linstrom and W.G. Mallard Eds. *NIST Chemistry WebBook, NIST Standard Reference Database Number 69.* National Institute of Standards and Technology, Gaithersburg MD, 20899, http://webbook.nist.gov, 2017.

[3] U. Even, J. Jortner, D. Noy, N. Lavie, and C. Cossart-Magos. Cooling of large molecules below 1 K and He clusters formation. *J. Chem. Phys.*, 112(18):8068, May 2000.

[4] F. Filsinger, J. Küpper, G. Meijer, L. Holmegaard, J. H. Nielsen, I. Nevo, J. L. Hansen, and H. Stapelfeldt. Quantum-state selection, alignment, and orientation of large molecules using static electric and laser fields. *J. Chem. Phys.*, 131(6):064309, 2009.

[5] R. Bacis, M. Broyer, S. Churassy, J. Vergès, and J. Vigué. eQq measurements in the X, 1g, $O_g^+$ and B state of $I_2$: A test of the electronic molecular eigenfunctions. *J. Chem. Phys.*, 73:2641, 1980.

[6] Chuan-Cun Shu, Esben F. Thomas, and Niels E. Henriksen. Femtochemistry in the electronic ground state: Dynamic stark control of vibrational dynamics. *Chem. Phys. Lett.*, 683:234–239, 2017.

[7] G. Maroulis. Accurate dipole polarizability for $Cl_2(X^1\Sigma_g^+)$. *Mol. Phys.*, 77:1085, 1992.

[8] G. Maroulis, C. Makris, U. Hohm, and D. Goebel. Electrooptical properties and molecular polarization of iodine, $I_2$. *J. Phys. Chem. A*, 101:953, 1997.

[9] N. C.-M. Bartlett, J. Jankunas, R. N. Zare, and J. A. Harrison. Time-dependent depolarization of aligned $D_2$ caused by hyperfine coupling. *Phys. Chem. Chem. Phys.*, 12:15689–15694, 2010.
